# Supplementary material for: Audio Retrieval with WavText5K and CLAP Training
Source: arXiv:2209.14275 source file (2022-09-28)
Supplement: Supplementary file 1 [file appendix.tex]

\section{Training datasets} \label{appendix: training datasets}

\noindent \textbf{FSD50k}~\cite{fsd50k} is a sound event classification dataset with audio clips from freesound.org. The duration of the clips ranges from 0.3 to 30 seconds. We used the ~36k clips from training and validation. We constructed the caption for each clip by concatenating the two sentences the associated title and description in the metadata. We ignored the class label. \\
\textbf{ClothoV2} \cite{clotho} is an audio captioning dataset consisting of ~7k audio clips. The duration of the clips range from 15 to 30 seconds. Each clip has 5 captions annotated by different participants. Thus, we created 5 pairs for each clip extending the number of audio-text pairs by 5 times. \\
\textbf{AudioCaps} \cite{audiocaps} is an audio captioning dataset consisting of ~46k audio clips from AudioSet. The duration of the clips is 10 seconds. Each clip has a caption annotated via crowd-sourcing. \\
\textbf{MACS} \cite{macs} is an audio captioning dataset consisting of ~4k audio clips. The duration of the clips is 10 seconds. Each clip is captioned by multiple participants. Similar to ClohtoV2, we paired the same audio with a each of their associated captions to create a larger set of pairs consisting of ~17k. 
At the time of downloading the datasets, not all clips were available from the web links.

\begin{table}[ht]
\center
\begin{tabular}{lccc} \hline
Dataset & Pairs & \makecell{Unique\\ audios} & \makecell{Unique \\captions} \\ \hline
FSD50k & 36,796 & 36,796 & 36,796 \\
ClothoV2 & 29,646 & 5,929 & 29,646 \\
AudioCaps & 44,292 & 44,292 & 44,292 \\
MACS & 17,276 & 3,930 & 17,276 \\ \hline
 & 128,010 & 90,947 & 128,010 \\ \hline
\end{tabular}
\caption{\label{table: training dataset}
Training dataset statistics. \vspace{-0.08in}}
\end{table}

\begin{table*}[ht]
\small
\center
\begin{tabular}{ccccccccc}\hline
 Domain & Dataset & Files & Dur. (secs) & Classes & Metric & Setup \\ \hline
\multirowcell{5}{
 Sound Event  \\ Classification (SEC)} & ESC50 & 2k & 5 & 50 & ACC & 5 folds \\
 & FSD50K & ~51k & 0.3 - 30 & 200 & mAP & train/val/test \\
 & UrbanSound8K & ~8k & $\leq$ 4 & 10 & ACC & 10 folds \\
 & DCASE2017 Task4 & 52k & 10 & 17 & ACC & train/val/test \\
 & AudioSet & $\sim$2M & 10 & 527 & mAP & train/val/test \\ \hline
% Acoustic \\ Scenes & Some dataset &  &  &  & ? &  \\ \hline
\multirowcell{5}{Music} & GTZAN Music Speech & 120 & 30 & 2 & ACC & 10 folds \\
 & GTZAN Music Genre & 1k & 30 & 10 & ACC & 10 folds \\
 & Mridangam Stroke & ~7k & 0.81 & 10 & ACC & 5 folds \\
 & Mridangam Tonic & ~7k & 0.81 & 6 & ACC & 5 folds \\ \hline
\makecell{Instrument \\ Classification} & \makecell{Beijing Opera \\ Percussions} & 236 & 4.77 & 4 & ACC & 5 folds \\ \hline
\makecell{Acoustic Scene \\ Classification} & TUT 2017 & 6.3k & 10 & 15 & ACC & train/val/test \\ \hline
\multirowcell{2}{Emotion \\ Recognition} & CREMA-D & ~7k & 5 & 6 & ACC & 5 folds \\
 & RAVDESS & ~2.5k & $\leq$ 5 & 8 & ACC & 5 folds \\ \hline
% Bio \\ Acoustics & Beehive states & 930 & 600 & 2 & ACC & train/val/test \\ \hline
Keyword \\ Spotting & Speech Commands & 100k & 1 & 12 & ACC & train/val/test \\ \hline
\makecell{Vocal Sound \\ Classification} & \makecell{Vocal Sound} & ~21k & 5 & 6 & ACC & train/val/test \\ \hline
Speaker Counting & LibriCount 10 & 5k & 5 &  11 & ACC & 5 folds \\\hline
\end{tabular}
\caption{\label{table: downstream datasets}
Details from the 16 datasets used as Downstream Tasks.
}
\end{table*}

\section{Downstream datasets} \label{appendix: downstream datasets}
\vspace{-0.05in}
\textbf{ESC50} is an environmental classification dataset comprising of 50 events. The dataset consists of 2k files of 5 seconds each. The evaluation setup is 5 fold cross validation and the evaluation metric is accuracy. \\
\textbf{FSD50K} is a sound event classification dataset comprising of 200 events. The dataset consists of 51k files ranging from 0.3 to 30 seconds each. The evaluation setup is train/val/test and the evaluation metric is mAP. \\
\textbf{UrbanSound8K} is urban sound classification dataset comprising of 10 sounds. The dataset consists of 8k files of ~4 seconds each. The evaluation setup is 10 fold cross validation and the evaluation metric is accuracy. \\
\textbf{DCASE2017 Task4} is a sound event classification dataset comprising of 17 sounds recorded in domestic environment. The dataset consists of ~30k files of 10 seconds each. The evaluation setup is train/val/test and the evaluation metric is accuracy. \\
\textbf{AudioSet} is a sound event classification dataset comprising of 527 sounds from YouTube videos. The dataset consists of ~2M files of 10 seconds each. The evaluation setup is train/val/test and the evaluation metric is accuracy. \\
\textbf{TUT 2017} is an acoustic scene classification dataset comprising of 15 acoustic scenes in both outdoor and indoor environment. The dataset consists of ~52k files of 10 seconds each. The evaluation setup is train/val/test and the evaluation metric is accuracy.\\ 
\textbf{GTZAN Music Speech} is a binary classification dataset where the aim is to distinguish between human speech and music. The dataset consists of 120 files of 30 seconds each. The evaluation setup is 10 fold cross validation and the evaluation metric is accuracy. \\
\textbf{GTZAN Genres} is music genre classification dataset comprising of 10 genres. The dataset consists of 1k files of 30 seconds each. The evaluation setup is 10 fold cross validation and the evaluation metric is accuracy. \\
\textbf{Mridangam Stroke} is music stroke classification dataset comprising of 10 strokes from Mridangam (pitched percussion instrument). The dataset consists of 1k files of 0.81 seconds each. The evaluation setup is 5 fold cross validation and the evaluation metric is accuracy. \\
\textbf{Mridangam Tonic} is music tonic classification dataset comprising of 6 tonics from Mridangam (pitched percussion instrument). The dataset consists of 1k files of 0.81 seconds each. The evaluation setup is 5 fold cross validation and the evaluation metric is accuracy. \\
\textbf{Beijing Opera Percussions} is an instrument classification dataset comprising of 4 percussion instruments from Beijing Opera. The dataset consists of 236 files of 4.77 seconds each. The evaluation setup is 5 fold cross validation and the evaluation metric is accuracy. \\
\textbf{CREMA-D} is an emotion recognition dataset comprising of 6 emotions. The dataset consists of ~7k files of 5 seconds each. The evaluation setup is 5 fold cross validation and the evaluation metric is accuracy. \\
\textbf{RAVDESS} is an emotion recognition dataset comprising of 8 emotions. The dataset consists of ~2.5k files of 5 seconds each. The evaluation setup is 5 fold cross validation and the evaluation metric is accuracy. \\
\textbf{Speech Commands V2} is an keyword spotting dataset comprising of 13 commands. The dataset consists of 100k files of 1 seconds each. The evaluation setup is train/val/test and the evaluation metric is accuracy.\\
\textbf{Vocal Sound} is a human vocal sound classification dataset comprising of 6 vocalizations. The dataset consists of 21k files of 5 seconds each. The evaluation setup is train/val/test and the evaluation metric is accuracy.\\
\textbf{LibriCount} is a speaker count estimation dataset comprising of simulated cocktail party environment audios consisting of 0 to 10 speakers. The dataset consists of 5k files of 5 seconds each. The evaluation setup is 5 fold cross validation and the evaluation metric is accuracy. \\

\begin{table*}[ht]
\small
\center
\begin{tabular}{c|cccc|cccc} \hline
\small
 & \multicolumn{4}{c|}{Sound Event Classification} & \multicolumn{4}{c}{Music} \\\hline
Model & ESC50 & FSD50K & US8K & \makecell{DCASE17 \\ Task 4} & \makecell{Music \\ Speech} & \makecell{Music \\ Genres} & \makecell{Mri. \\ Stroke} & \makecell{Mri. \\ Tonic}\\ \hline
YAMNet & 0.8375 & - & - & -   & 0.969 & 0.847 & - & - \\
Open L3 & 0.7505 & 0.4470 & 0.7823 & -   & 0.969 & 0.879 & 0.9666 & 0.9369 \\
Wav2CLIP & 0.7589 & 0.3617 & - & -   & 0.946 & 0.748 & 0.9471 & 0.8289 \\
PaNN & 0.9085 & - & - & -   & 0.992 & 0.860 & 0.9390 & 0.8244 \\
Wav2Vec2 & 0.5610 & 0.1164 & - & -   & 0.946 & 0.780 & 0.9432 & 0.8283 \\ 
CLAP (S) & 0.9310 & 0.5905 & 0.8389 & 0.5330  & 1.0 & 0.7930 & 0.7754 & 0.6391 \\
CLAP (F) & 0.9670 & 0.5859 & 0.8796 & 0.5938  & 1.0 & 0.9130 & 0.9794 & 0.9534  \\ \hline
\end{tabular}
\smallskip
\center
\begin{tabular}{c|c|c|cc|c|c|c} \hline
\small
& \multicolumn{1}{c|}{\makecell{Instrument\\Classification}} & \multicolumn{1}{c|}{\makecell{Acoustic Scene\\Classification}} & \multicolumn{2}{c|}{Emotion Recognition} & \multicolumn{1}{c|}{\makecell{Keyword \\ Spotting}} & \makecell{Human \\ Vocalization} & \multicolumn{1}{c}{\makecell{Speaker \\ Estimation}} \\ \hline
Model & \makecell{Beijing \\ Opera} & \makecell{TUT 2017} & \makecell{CRE\\MA-D} & \makecell{RAV\\DESS} &  \makecell{Speech \\ Comm.} & \makecell{Vocal\\Sounds} & \makecell{Libri \\ Count} \\ \hline
YAMNet & 0.941 & - & 0.453  & 0.479 & 0.4104 & - & 0.6526 \\
OpenL3 & 0.975 & - & 0.550  & 0.604 & 0.7634 & - & 0.6414 \\
Wav2CLIP & 0.936 & - & 0.512  & 0.684 & 0.3466 & - & 0.5276 \\
PaNN & 0.911 & - & 0.555  & 0.429 & 0.6182 & - & 0.6516 \\
Wav2Vec2 & 0.907 & - & 0.6562  & - & 0.8785 & - & 0.6921 \\
CLAP (S) & 0.7754 & 0.7099 & 0.2830 & 0.4515  & 0.3708 & 0.8411 & 0.5715 \\
CLAP (F) & 0.9026 & 0.7463 & 0.6834 & 0.6436  & 0.9683 & 0.9795 & 0.7783 \\ \hline
\end{tabular}
\caption{\label{table: shallow results}
CLAP's Supervised Feature Extraction (S) and Supervised Finetune (F) performance against SoTA models.
}
\end{table*}

\begin{table*}[ht]
\small
\center
\begin{tabular}{lll} \hline
Dataset & Audio captions \\ \hline
ClothoV2 & A bow playing a stringed instrument in a one note tone repeatedly before violins join to create the melody\\
ClothoV2 & An insect buzzing in the foreground as birds chirp in the background\\
ClothoV2  & A camp fire crackles as the flames burn branches and leaves \\
\hline
AudioCaps & Several sirens are wailing and a horn is honked twice \\
AudioCaps & Church bells chime loudly and repeatedly\\
AudioCaps & Beating drum getting faster than children voices and clapping then adult male voice \\ \hline
FSD50K & Water dripping in a cave or underground temple \\
FSD50K & Canada geese flying down and landing near a lakeshore. Recorded with an Olympus LS-14. \\
FSD50K & Leaves falling in a forest near a pond. Recorded in October 2017 in a German forest using a Zoom H2n. \\ \hline
MACS & Two people having a conversation nearby while a lot of adults  and a child talk far away \\
MACS & Birds are making a lot of noises and a distant child yells \\
MACS & Dog barks followed by adults talking and children voices \\ \hline
\end{tabular}
\caption{\label{table: caption example}
Randomly sampled raw captions from each dataset.
}
\end{table*}

\section{Discussion} \label{appendix: discussion}

\subsection{Batch size and CLAP performance}

Appropriate batch size is a key contributor in performance of any contrastive learning methods that uses positive-negative pairs. In computer vision literature, larger batch size has shown to improve performance \cite{radford2021learning, yuan2021florence, zhai2021lit}. 

We use Tesla V100 16 GB GPUs for this analysis. The number of GPUs used vary from 4 to 24 for batch size from 32 to 768. We measure the zero-shot performance by computing average performance across N downstream tasks listed in table \ref{table: downstream datasets}. Our findings also indicate that the larger batch size does lead to improved CLAP performance. However, we saw decreased performance with batch size of 768. This might be an anamoly in an increasing zero-shot performance trend. We leave the larger batch size investigation to future work. 

\begin{figure}[ht]
  \centering
     \includegraphics[width=2.5in]{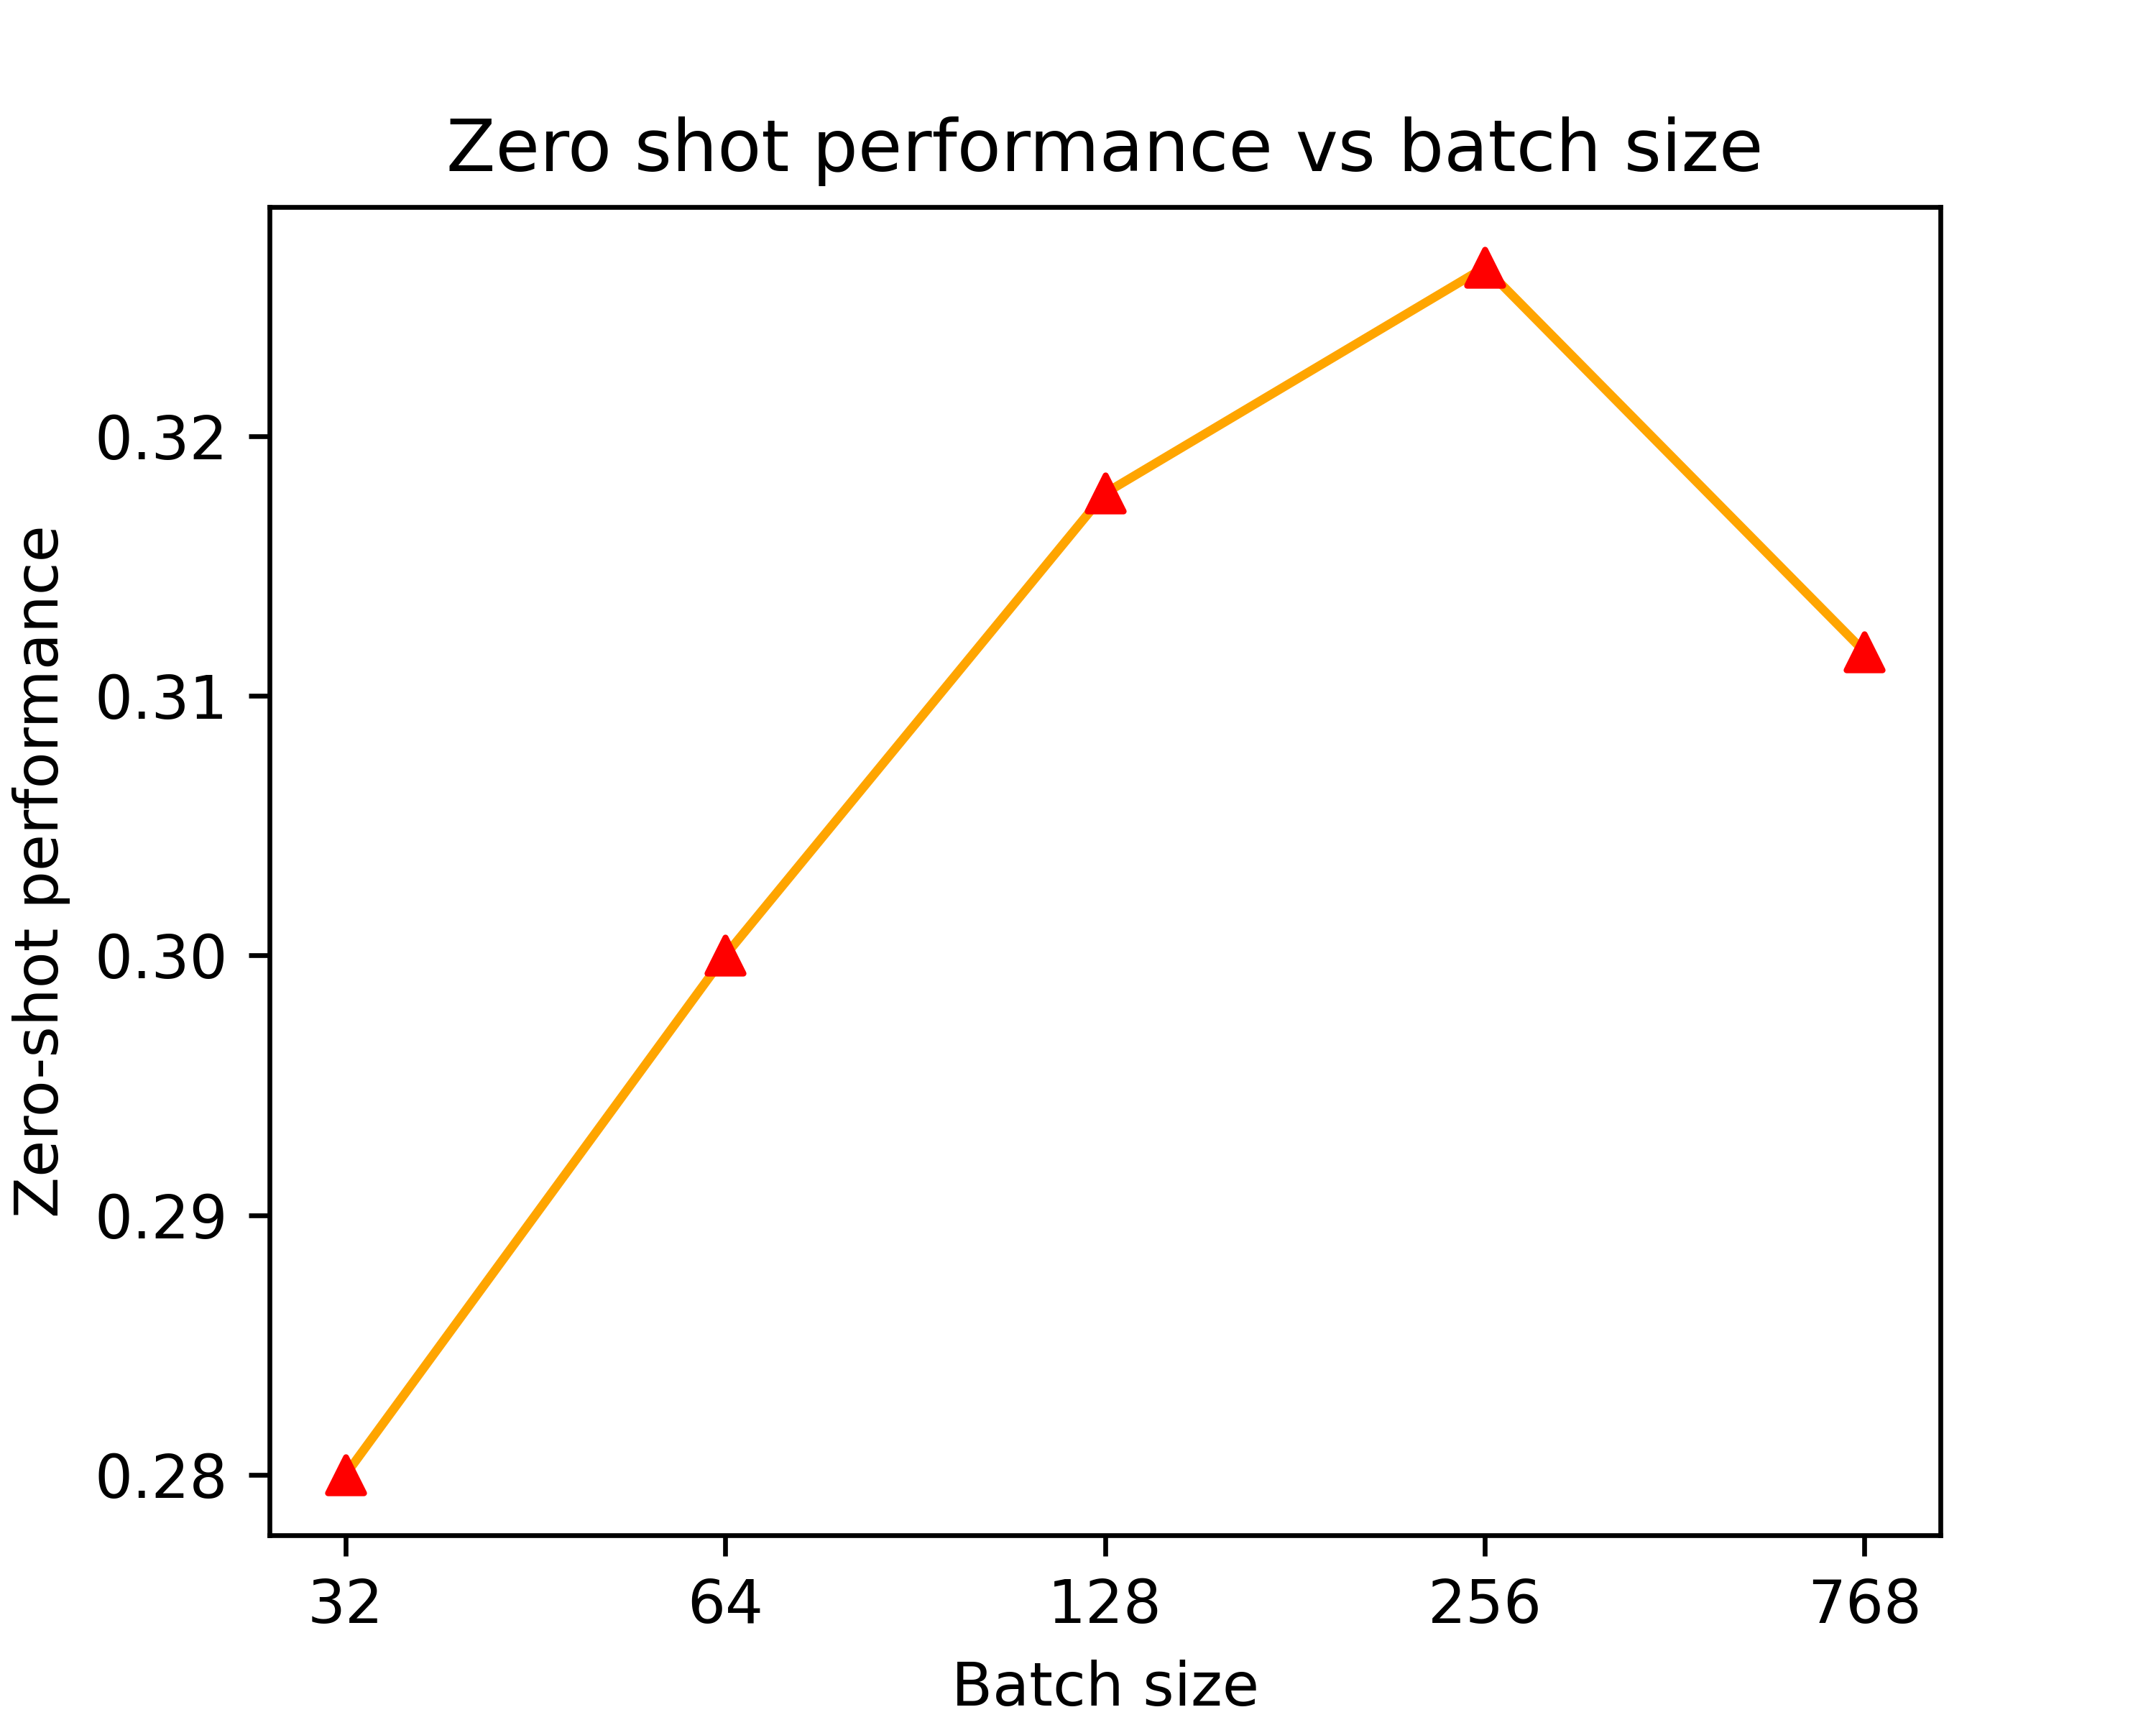}
     \caption{Effect of batch size on zero-shot performance}
     \label{fig:clap_batch_size}
\end{figure}

\subsection{Training with AudioSet}
AudioSet is a multilabled sound event dataset with ~2M audio clips, but it does not come with a text descriptions per clip, thus making it complicated to extract audio and text pairs for training. We tried constructing the text description with the title and the class label(s). However, adding about ~1.7M pairs to the existing 128k pairs resulted in a performance dropped in the overall zero-shot numbers. For example, ESC50 performance dropped from 82.6\% to 67.15\% acc and US8K dropped from 73.24\% to 70.93\% acc. Only Speech Commands V2 (SCV2) performance improved from 10\% to 15\% acc. Perhaps due to the large amount of audio containing speech in AudioSet. The quality of audio-text pairs is key in training CLAP. In AudioSet, often the YouTube titles and descriptions do not describe the acoustic content of the video segment under consideration but instead describe the video as a whole. More intelligent ways of generating descriptions can benefit CLAP training with AudioSet and other many similar datasets. In general, finding helpful training data for CLAP based on public datasets is difficult, thus relying on large-scale noisy pairs is the only scalable approach.

\section{Acknowledgements} \label{appendix: acknowledgements}
We thank Hamid Eghbalzadeh for early discussions and feedback.
